# Supplementary material for: PredBench: Benchmarking Spatio-Temporal Prediction across Diverse Disciplines
Source: arXiv:2407.08418 source file (2024-07-12)
Supplement: Supplementary file 2 [file repr_mcvd.tex]

\begin{table*}[t]

\setlength\tabcolsep{1pt}
\center
\vspace{-0.02cm}
\caption{\textbf{Reproduction results} of MCVD~\cite{voleti2022mcvd} on \textit{KTH}~\cite{schuldt2004kth} and \textit{BAIR}~\cite{ebert2017bair}.}
\label{tab:exp_std_weather}
\vspace{-0.3cm}
\begin{adjustbox}{max width=1.\columnwidth}
\begin{tabular}{l|c|cccccc|cccccc}
\toprule[1.3pt]
  \multirow{3}*{Method}
  &\multirow{3}*{Released Code}
  &\multicolumn{6}{c|}{KTH}
  &\multicolumn{6}{c}{BAIR}
  \\ 
  % \cline{6-11}

  & 
  & \multicolumn{2}{c}{\textbf{FVD}} & \multicolumn{2}{c}{\textbf{PSNR}} & \multicolumn{2}{c|}{\textbf{SSIM}}
  & \multicolumn{2}{c}{\textbf{FVD}} & \multicolumn{2}{c}{\textbf{PSNR}} & \multicolumn{2}{c}{\textbf{SSIM}}
  \\ 
  % \cline{6-11}

  &
  & \textbf{original} & \textbf{ours} 
  & \textbf{original} & \textbf{ours} 
  & \textbf{original} & \textbf{ours} 
  & \textbf{original} & \textbf{ours} 
  & \textbf{original} & \textbf{ours} 
  & \textbf{original} & \textbf{ours} 
  \\
  
\Xhline{0.5pt}

    MCVD & \href{https://github.com/voletiv/mcvd-pytorch}{GitHub}
    &  & 
    &  & 
    &  & 
    &  & 
    &  & 
    &  & 
    \\
    
\bottomrule[1.3pt]
\end{tabular}
\end{adjustbox}
\vspace{-0.5cm}
\end{table*}
